# Supplementary material for: Rectangular diagrams of surfaces: distinguishing Legendrian knots
Source: arXiv:1712.06366 ancillary file (2021-03-29)
Supplement: Supplementary file 1 [file program-description.pdf]

# A PYTHON CODE FOR SEARCHING ALL REALIZATIONS OF A DIVIDING CONFIGURATION

IVAN DYNNIKOV

This paper is supplementary to the work [2] where a new method to distinguish Legendrian knots is proposed. In many cases, to use the method requires an exhaustive search of certain combinatorial objects, which is often infeasible to perform manually. Here is provided a `Python` script that implements this exhaustive search, along with a description of the algorithm. The reader who wishes to use the script is encouraged to download the source files of the present preprint, among which he or she will find the `.py` file with the program along with a supplementary `.txt` file. The script is compatible with both `Python 2` and `Python 3`.

Note, however, that the program does not have any helpful user interface. To run the script for initial data other than those included in the script the lines 1 through 4 should be replaced accordingly.

## 1. THE PROBLEM

Here we describe briefly the combinatorial problem solved by the script.

By  $\mathbb{S}^1$  we denote the circle  $\mathbb{R}/(T\mathbb{Z})$ , where the period  $T$  is a positive real number, which will be specified later. We use the notation  $\langle \rangle$  for the cyclic order on  $\mathbb{S}^1$ . More precisely, if  $x_1, \dots, x_n \in \mathbb{S}^1$ , then  $\langle x_1 x_2 \dots x_n \rangle$  stands for the following statement: there exist  $a_1, a_2, \dots, a_n \in \mathbb{R}$  such that  $a_1 < a_2 < \dots < a_n < a_1 + T$  and  $x_i = a_i + T\mathbb{Z}$ ,  $i = 1, 2, \dots, n$ . If  $x, y$  are distinct points of  $\mathbb{S}^1$  we also use the following notation:

$$[x; y] = \{z \in \mathbb{S}^1 : \text{not } \langle xyz \rangle\}, \quad (x; y) = \{z \in \mathbb{S}^1 : \langle xzy \rangle\}.$$

By  $\mathbb{T}^2$  we denote the torus  $\mathbb{S}^1 \times \mathbb{S}^1$ . For any  $x, y \in \mathbb{S}^1$ , the subset  $m_x = \{x\} \times \mathbb{S}^1 \subset \mathbb{T}^2$  (respectively,  $\ell_y = \mathbb{S}^1 \times \{y\} \subset \mathbb{T}^2$ ) is called *a meridian* (respectively, *a longitude*) of the torus  $\mathbb{T}^2$ .

**Definition 1.** A *rectangle* in  $\mathbb{T}^2$  is a subset of the form  $[x_1; x_2] \times [y_1; y_2] \subset \mathbb{T}^2$ , where  $x_1 \neq x_2$ ,  $y_1 \neq y_2$ . The points  $(x_1, y_1)$ ,  $(x_1, y_2)$ ,  $(x_2, y_1)$ , and  $(x_2, y_2)$  are called, respectively, *the bottom left vertex*, *the top left vertex*, *the bottom right vertex*, and *the top right vertex* of  $r$ .

**Definition 2.** Two rectangles  $r_1 = [x'_1; x''_1] \times [y'_1; y''_1]$  and  $r_2 = [x'_2; x''_2] \times [y'_2; y''_2]$  are said to be *compatible* with one another if one of the following cases occurs:

- (1)  $r_1 \cap r_2 \subset \{x'_1, x''_1\} \times \{y'_1, y''_1\}$  (which is equivalent to  $r_1 \cap r_2 \subset \{x'_2, x''_2\} \times \{y'_2, y''_2\}$ );
- (2)  $\langle x'_1 x'_2 x''_2 x''_1 \rangle$  and  $\langle y'_1 y'_2 y''_2 y''_1 \rangle$ ;
- (3)  $\langle x'_2 x'_1 x''_1 x''_2 \rangle$  and  $\langle y'_2 y'_1 y''_1 y''_2 \rangle$ .

In other words, two compatible rectangles may be disjoint, may share one, two, or four vertices and nothing else, or may overlap forming a ‘plaster cross’, see Figure 1.

**Definition 3.** A finite collection  $\Pi$  of pairwise compatible rectangles in  $\mathbb{T}^2$  is called *a rectangular diagram of a surface* if every meridian and every longitude of the torus contains at most two points  $p$  such that  $p$  is a vertex of exactly one rectangle in  $\Pi$ .

Meridians and longitudes of  $\mathbb{T}^2$  containing at least one side of a rectangle  $r \in \Pi$  are called *occupied levels* of  $\Pi$ .

Two rectangular diagrams of a surface  $\Pi, \Pi'$  are said to be *combinatorially equivalent* (or to have the same *combinatorial type*) if there exist orientation preserving homeomorphisms  $\phi, \psi :$

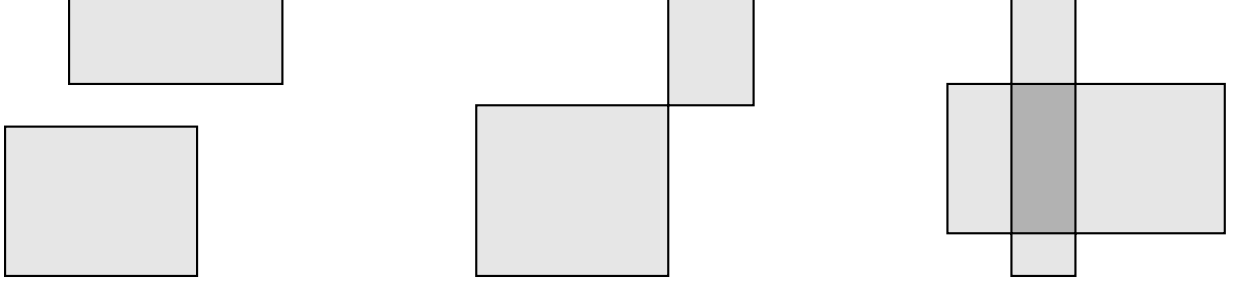

FIGURE 1. Compatible rectangles

$\mathbb{S}^1 \rightarrow \mathbb{S}^1$  such that the homeomorphism  $\phi \times \psi : \mathbb{T}^2 \rightarrow \mathbb{T}^2$  takes  $\Pi$  to  $\Pi'$  (meaning that  $\Pi' = \{(\phi \times \psi)(r) : r \in \Pi\}$ ).

In order to draw a rectangular diagram of a surface we cut the torus  $\mathbb{T}^2$  along a meridian and a longitude to get a square. As a consequence some rectangles are cut into two or four parts.

When two or more rectangles overlap we draw them so that some rectangles appear lying over others. The rule is this: if  $\langle x'_1 x'_2 x''_2 x''_1 \rangle$  and  $\langle y'_2 y'_1 y''_1 y''_2 \rangle$ , then  $[x'_2; x''_2] \times [y'_2; y''_2]$  lies over  $[x'_1; x''_1] \times [y'_1; y''_1]$ . The reason for this is explained in [1, 2].

An example of a rectangular diagram of a surface is shown in Fig. 2.

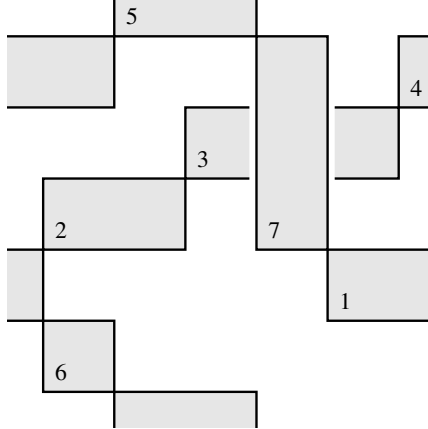

FIGURE 2. A rectangular diagram of a surface

For two compatible rectangles  $r_1$  and  $r_2$  we write  $r_1 \cdot r_2$  (respectively,  $r_1 \cdot r_2$ ) if the top right vertex of  $r_1$  coincides with the bottom left vertex of  $r_2$  (respectively, the bottom right vertex of  $r_1$  coincides with the top left vertex of  $r_2$ ). (Note that all four relations  $r_1 \cdot r_2$ ,  $r_2 \cdot r_1$ ,  $r_1 \cdot r_2$ , and  $r_2 \cdot r_1$  may hold simultaneously.)

It follows from the definition of a rectangular diagram of a surface that, if  $\Pi$  is such a diagram, each vertex of a rectangle  $r \in \Pi$  is shared with at most one rectangle  $r' \in \Pi$  distinct from  $r$ . This means that, for any  $r_1, r_2, r_3 \in \Pi$ , we have  $r_1 \cdot r_2 = r_1 \cdot r_3 \Rightarrow r_2 = r_3$ , etc.

**Definition 4.** Let  $\Pi$  be rectangular diagram of a surface. By a  $\cdot$ -chain of  $\Pi$  (respectively, a  $\cdot$ -chain) we call a maximal sequence  $r_1, r_2, \dots, r_k$  of rectangles of  $\Pi$  such that  $r_1, \dots, r_{k-1}$  are pairwise distinct and for all  $i = 1, \dots, k-1$  we have  $r_i \cdot r_{i+1}$  (respectively,  $r_i \cdot r_{i+1}$ ). Note that we allow  $r_k$  to coincide with  $r_1$ .

Let  $A$  (respectively,  $B$ ) be a maximal collection of pairwise disjoint  $\cdot$ -chains (respectively,  $\cdot$ -chains) of  $\Pi$ , and let  $f : \{1, \dots, n\} \rightarrow \Pi$  be a bijection. Replace each rectangle  $r$  in every chain

in  $A$  and  $B$  by the respective number  $f^{-1}(r)$ . The obtained pair of collections of sequences is called a *dividing code* of  $\Pi$ .

For instance, the following is a dividing code of the diagram shown in Figure 2:

$$(1) \quad \left( \{(1, 2, 3, 4, 5), (6), (7)\}, \{(1, 7, 5, 6, 1), (2), (3), (4)\} \right)$$

A dividing code of a rectangular diagram of a surface  $\Pi$  does *not*, in general, determine the combinatorial type of  $\Pi$ . What it does determine is the combinatorial structure of *the canonic dividing configuration* of the surface  $\widehat{\Pi}$  associated with  $\Pi$ . For the definitions of these the reader is referred to [2].

The problem solved by the script provided below is the following one:

*find all rectangular diagrams of a surface with the given dividing code.*

In terms of [2] this means that the script finds all *realizations* of the given *dividing configuration*. For this reason the two lists of sequences that contain the initial data are named `dividing1` and `dividing2`. The `dividing1` list encodes all the  $\cdot$ -chains, and the `dividing2` list encodes all the  $\cdot$ -chains in the dividing code. The order of entries in each list does not matter. The reader who wishes to run the script for different initial data should not forget to include one-element sequences, if there are any, in these lists.

For instance, to run the program for the dividing code (1) one should replace lines 1 through 4 of the script below with

```
dividing1=[(1,2,3,4,5),(6,),(7,)]
dividing2=[(1,7,5,6,1),(2,),(3,),(4,)]
```

In practice, one does not need to find all realizations of the given dividing configuration, but only those that are *proper* (see [2]). Deciding which realizations are proper is a hard problem in general, and the present script does not try to solve it. However, it does sort out certain realizations using the criterium that we explain below.

**Definition 5.** Let  $\Pi$  be a rectangular diagram of a surface. *The boundary  $\partial\Pi$  of  $\Pi$*  is the set of all points  $v \in \mathbb{T}^2$  such that  $v$  is a vertex of exactly one rectangle in  $\Pi$ .

The boundary  $\partial\Pi$  of a rectangular diagram of a surface is a rectangular diagram of a link. Each meridian and each longitude meets  $\partial\Pi$  in either no or exactly two points. Pairs of points of  $\partial\Pi$  that lie on the same meridian (respectively, the same longitude) are called *vertical edges* (respectively, *horizontal edges*) of  $\partial\Pi$ .

The script was initially intended to be used in the situation when the boundary of any proper realization does not admit any simplification by elementary moves. For this reason, the script is designed to sort out any realization  $\Pi$  if its boundary fits the following definition, in which case it is obviously simplifiable.

**Definition 6.** A rectangular diagram of a link  $R$  is said to be *destabilizable* if there exists a rectangle  $r = [\theta_1; \theta_2] \times [\varphi_1; \varphi_2]$  such that  $R \cap r$  consists of exactly three vertices of  $r$ , and at least one of the sets  $(\theta_1; \theta_2) \times \mathbb{S}^1$  and  $\mathbb{S}^1 \times (\varphi_1; \varphi_2)$  is disjoint from  $R$ .

The user who wants to see all realizations in the output, including those with destabilizable boundary, should just comment out the lines 272–293 of the program.

## 2. THE ALGORITHM

The program consists of four logical parts: preparation of a convenient presentation of the data, preparation of the set of conditions against which the realizations are checked during construction, the actual exhaustive search, and conversion of the output into pictures.

To run the search we create objects representing rectangles and occupied levels of the sought-for diagrams. These objects will be referred to as *abstract rectangles* and *abstract occupied levels*, respectively. Each abstract rectangle  $\mathbf{r}$  is attributed references to the abstract occupied levels corresponding to the sides of the rectangle represented by  $\mathbf{r}$ , and vice versa. This information is easily extracted from the given dividing code.

Later, during the search, abstract occupied levels are assigned concrete *positions*, which are represented by integers  $0, 1, 2, \dots$ . We have two independent lists, one for vertical and one for horizontal occupied levels. When all abstract occupied levels are assigned positions all the abstract rectangles get associated with actual rectangles in  $\mathbb{T}^2$ , and if these rectangles are pairwise compatible, we get a realization. The period  $T$  is thought of as being assigned a sufficiently large value, namely, larger than the number of occupied levels of each direction. The concrete value of  $T$  plays no role and is never used during the implementation of the program.

The next task is to create a list of conditions such that their conjunction is necessary and sufficient for a position assignment to yield a realization of the given dividing code. The conditions we deal with either have the form  $\langle xyz \rangle$ , in which case they are referred to as *first order conditions*, or the form  $\langle abc \rangle \Rightarrow \langle xyz \rangle$ , in which case they are called *second order conditions*, where  $x, y, z$  are abstract occupied levels of the same direction, and  $a, b, c$  are abstract occupied levels of the perpendicular direction. The conditions can be evaluated when the involved abstract occupied levels are assigned concrete positions, by substituting the positions for the corresponding abstract occupied levels.

The first order conditions come from the cyclic order of vertices of the rectangles lying on the same occupied level. For every occupied level, this cyclic order is extracted from the information about the incidence between rectangles and occupied levels.

The second order conditions come from demanding that the vertices of any rectangle do not appear in the interior of another one. If the diagram contains a rectangle  $[\theta_1; \theta_2] \times [\varphi_1; \varphi_2]$  and another rectangle has a vertex at  $(\theta_3; \varphi_3)$ , then the corresponding second order conditions are  $\langle \theta_1 \theta_3 \theta_2 \rangle \Rightarrow \langle \varphi_2 \varphi_3 \varphi_1 \rangle$  and  $\langle \varphi_1 \varphi_3 \varphi_2 \rangle \Rightarrow \langle \theta_2 \theta_3 \theta_1 \rangle$ .

The list of conditions get modified back and forth many times during the search as described below. At every moment, each abstract occupied level that is not assigned a concrete position is attributed a list of all *available places* where we can put this level. Available places are those where the putting of the occupied level would comply with all currently known first order conditions, and such that they have not already been tried for the current configuration of other occupied levels.

The actual search consists in repeating the following steps in a loop.

**Step 1:** Pick an abstract occupied level that is currently not assigned any concrete position, and make an *assumption* about its position (relative to the abstract occupied levels of the same direction which have been assigned positions earlier) picking an item from the corresponding list of available places. Make a record on the *stack of actions* about this assumption. If the list of available places has more than one entry, the assumption is referred as *essential*.

**Step 2:** Whenever we have a second order condition  $\langle abc \rangle \Leftrightarrow \langle xyz \rangle$  such that all three abstract occupied levels  $a, b, c$  have been assigned a position and  $\langle abc \rangle$  evaluates to **True**, turn  $\langle xyz \rangle$  into a first order condition. All such modifications of the condition list are recorded on the action stack.

**Step 3:** For each abstract occupied level that is currently not assigned a position, adjust the list of available places for this occupied level according to the change in the list of first order conditions. Make a record about these changes on the action stack.

**Step 4:** If there are no abstract occupied levels left without a position assignment, we have found a realization. Check whether the boundary of the obtained diagram is destabilizable, and if not, append the diagram to the realization list. After that proceed to Step 6.

**Step 5:** Unless there is an abstract occupied level that has empty list of available positions, skip the next step and proceed to Step 1.

**Step 6:** Undo the last actions recorded on the action stack until an essential assumption is encountered or the stack goes empty. In the latter case, stop the search. Otherwise, adjust the list of available positions for the abstract occupied level on which the last essential assumption was made so as to prevent this assumption from being made again in the current configuration. As always, make a corresponding record on the action stack.

### 3. THE SCRIPT

Here follows the initial data.

```
1 dividing1=[(1,2,3,4),(5,6),(7,8,9,10,11,12),(13,14),
2            (15,16),(17,18),(19,20),(21,22)]
3 dividing2=[(10,3,22,19,8,15,2,11,14,17,16,5,12,1,18,
4            13,6,7,20,21,4,9)]
```

As noted above, in order to run the algorithm for other dividing configurations, lines 1–4 must be replaced.

The following are some dictionaries that serve for better readability and do not ever change.

```
5 opposite={'right':'left','left':'right','top':'bottom','bottom':'top'}
6 forward={'right':'ne','left':'nw','top':'ne','bottom':'se'}
7 backward={'right':'se','left':'sw','top':'nw','bottom':'sw'}
```

The following function returns True if and only if the condition  $\langle ijk \rangle$  holds true.

```
8 def even(i,j,k):
9     return (i<j)^(j<k)^(i<k)
```

Objects of the following class, named `triple`, represent conditions of the form  $\langle x_1x_2x_3 \rangle$  with  $x_1$ ,  $x_2$ , and  $x_3$  abstract occupied levels. The attribute `level` counts how many elements of the triple are currently assigned a concrete position, and takes, therefore, integer values from 0 to 3.

First order conditions will be represented by `triple` objects with the `must_hold` attribute set to True. To represent a second order condition  $\langle abc \rangle \Rightarrow \langle xyz \rangle$  we include  $\langle xyz \rangle$  into consequences of  $\langle abc \rangle$ .

```
10 class triple(tuple):
11     def __init__(self,*args):
12         self.level=0
13         self.must_hold=False
14         self.consequences=[]
```

In order to be able to compare conditions quickly we write them in a canonical form, which is computed by the following function.

```
15 def normalize(a):
16     (x,y,z)=a
17     b=(x.label,y.label,z.label)
```

```

18     j=b.index(min(b))
19     return triple(a[j:]+a[:j])

```

The following function decomposes any condition on the form  $\langle x_1x_2x_3 \dots x_n \rangle$  into a conjunction of ternary conditions  $\langle x_ix_jx_k \rangle$ , which are listed in the output. This is done by recursively using the equivalence  $\langle x_1x_2x_3 \dots x_n \rangle \Leftrightarrow \langle x_1 \dots x_j \rangle \& \langle x_j \dots x_n \rangle \& \langle x_1x_jx_n \rangle$ , where  $j = \lceil (n+1)/2 \rceil$ . Trivial conditions  $\langle x_kx_l \rangle$  are discarded.

```

20 def subdivide(a):
21     if len(a)<3: return []
22     s=[a]
23     i=0
24     while i<len(s):
25         x=s[i]
26         if len(x)==3:
27             s[i]=normalize(x)
28             i+=1
29             continue
30         j=len(x)//2
31         x1=(x[0], x[j], x[-1])
32         x2=x[:j+1]
33         x3=x[j:]
34         del(s[i])
35         s.append(x1)
36         s.append(x2)
37         if len(x3)>2: s.append(x3)
38     return s

```

Abstract rectangles are represented by objects of the class `rectangle`, which is defined next. The objects are initially created with the only attribute called `label`, which is used for identification. Later on these objects will be also assigned optional attributes named `nw`, `ne`, `sw`, and `se`, which hold references to the rectangles that share a vertex with the given one, and also obligatory attributes named `left`, `right`, `top`, and `bottom`, which hold references to the occupied levels containing the respective sides of the rectangle.

```

39 class rectangle(object):
40     registry=dict()
41     def __init__(self,i):
42         self.label=i
43         rectangle.registry[i]=self

```

Abstract occupied levels are represented by objects of the class `position`, which is defined below.

```

44 class position(object):
45     def __init__(self, l0, side0):

```

The `__init__()` function receives two arguments: `l0` and `side0` whose meaning is as follows. The created `position` class object represents the occupied level that contains the `side0` side of the rectangle having label `l0`.

A number of attributes are assigned initial values:

- `conditions` is the list of all `triple` class objects involving the given `position` class object;
- `options` is the list of currently available places for the respective occupied level;

- `place` is set to an integer when a concrete place for the respective occupied level has been chosen, and to `None` otherwise;
- `edgelevel` is a Boolean that indicates whether or not the corresponding occupied level contains an edge of the boundary of the diagram.

The values of these attributes will vary in the course of the program implementation.

```

46         self.conditions=[]
47         self.options=[0]
48         self.place=None
49         self.edgelevel=True

```

The abstract occupied levels are also assigned labels, which have been helpful for debugging and are useful for analyzing the search process. Note that `position.registry` refers to nothing, but the `position` class is used only through two subclasses, `hposition` and `vposition` (see below), which do have the `registry` attribute.

```

50         i=len(self.__class__.registry)
51         self.label=i
52         self.__class__.registry[i]=self

```

Now the rectangle having label 10 is being linked to the `position` class object that is being created.

```

53         r=rectangle.registry[10]
54         side=side0
55         r.__dict__[side]=self

```

Any `position` object is also equipped with a list of all the (abstract) rectangles that have one of their sides on the corresponding occupied level. The rectangles are listed in the order their sides appear on this occupied level, from left to right if the occupied level is horizontal, and from bottom to top if the occupied level is vertical. Each rectangle is linked to the occupied level through the respective attribute (`left`, `right`, `top`, or `bottom`).

In order to create the list we start from the rectangle labeled 10 and proceed in the ‘forward’ direction until one of the following two events occur.

- (1) We make a full round along the occupied level and come back to the rectangle labeled 10. This means that the occupied level does not contain boundary vertices of the diagram, and we have visited all rectangles having a side on the currently examined occupied level.
- (2) We arrive at a boundary vertex. In this case, we have to start from the rectangle labeled 10 again and proceed in the ‘backward’ direction until we arrive at another boundary vertex.

```

56         rectangles=[r]
57         self.rectangles=rectangles
58         while True:
59             direction=forward[side]
60             try:
61                 r=r.__dict__[direction]
62                 if r.label==10:
63                     self.edgelevel=False
64                     return None
65                 side=opposite[side]
66                 rectangles.append(r)

```

```

67         r.__dict__[side]=self
68     except KeyError:
69         break
70     r=rectangles[0]
71     side=side0
72     while True:
73         direction=backward[side]
74         try:
75             r=r.__dict__[direction]
76             side=opposite[side]
77             rectangles.insert(0,r)
78             r.__dict__[side]=self
79         except KeyError:
80             break

```

Definition of the position class is now complete. Here are two subclasses we actually use.

```

81 class hposition(position):
82     registry=dict()
83 class vposition(position):
84     registry=dict()

```

During the search, we are going to consider a lot of cases by making assumptions and deriving consequences. Once we arrive at a contradiction or find a new realization we raise an exception called Contradiction.

```

85 class Contradiction(Exception):
86     pass

```

Now we create all necessary rectangle class objects.

```

87 for s in dividing1:
88     for i in s:
89         if not i in rectangle.registry.keys():
90             rectangle(i)

```

Any two rectangles sharing a vertex (or two vertices, or four vertices) are linked to each other by means of the `ne`, `nw`, `se`, `sw` attributes. For instance, if the top right (that is, NE) vertex of a rectangle `r1` coincides with the bottom left (that is, SW) vertex of a rectangle `r2`, we put `r1.ne=r2` and `r2.sw=r1`.

```

91 for s in dividing1:
92     for i in range(0,len(s)-1):
93         k=s[i]
94         m=s[i+1]
95         r1=rectangle.registry[k]
96         r2=rectangle.registry[m]
97         r1.ne=r2
98         r2.sw=r1
99 for s in dividing2:
100     for i in range(0,len(s)-1):
101         k=s[i]
102         m=s[i+1]
103         r1=rectangle.registry[k]
104         r2=rectangle.registry[m]

```



```

105         r1.nw=r2
106         r2.se=r1

```

Now we create all necessary `hposition` and `vposition` objects. As we have seen, their `__init__()` function makes all the necessary links between them and the rectangles.

```

107 for i in rectangle.registry:
108     r=rectangle.registry[i]
109     for side in ('right','left'):
110         if not side in r.__dict__:
111             hposition(i,side)
112     for side in ('top','bottom'):
113         if not side in r.__dict__:
114             vposition(i,side)

```

By this point, we have created all abstract occupied levels and all abstract rectangles, and also linked them to each other in all relevant ways. Next, we create lists of abstract horizontal and vertical edges (`he` and `ve`, respectively) and the list of first order conditions of the form  $\langle xyz \rangle$  that guarantee that vertices of rectangles do not appear in the interior of the sides of other rectangles (`restrictions`).

Each abstract horizontal edge is a triple  $(a, b, c)$  in which  $a$  is a `vposition` object representing the longitude containing the edge, and  $b, c$  are `hposition` objects each containing one of the two vertices of this edge. Symmetrically for vertical edges.

```

115 restrictions=[]
116 he=[]
117 for i in vposition.registry:
118     a=vposition.registry[i]
119     s=[]
120     for r in a.rectangles:
121         s.append(r.left)
122     if a.edgelevel:
123         s.append(a.rectangles[-1].right)
124     he.append((a,s[0],s[-1]))
125     restrictions+=subdivide(tuple(s))
126 ve=[]
127 for i in hposition.registry:
128     a=hposition.registry[i]
129     s=[]
130     for r in a.rectangles:
131         s.append(r.bottom)
132     if a.edgelevel:
133         s.append(a.rectangles[-1].top)
134     ve.append((a,s[0],s[-1]))
135     restrictions+=subdivide(tuple(s))
136 restrictions=list(set(restrictions))

```

All conditions of the form  $\langle xyz \rangle$  we have included so far into the `restrictions` list are going to be first order conditions. So, we mark them as such.

```

137 for t in restrictions:t.must_hold=True

```

The number of horizontal boundary edges (which is the same as the number of vertical edges) is assigned to `n`.



The following block (lines 182 through 195) is for a little bit of optimization. If  $\langle abc \rangle$  is a first order condition and  $\langle abc \rangle \Rightarrow \langle xyz \rangle$  is a second order condition then we may discard the latter and make  $\langle xyz \rangle$  a first order condition. The `triple` class objects that do not represent any first order condition or a part of a second order condition can be discarded. This allows sometimes to simplify the family of conditions operated during the search, but the script will work even if this block is removed.

```

182 checklist=list(restrictions)
183 while(len(checklist)>0):
184     t=checklist.pop(0)
185     if not t.must_hold and len(t.consequences)==0:
186         restrictions.remove(t)
187     if t.must_hold:
188         for t1 in t.consequences:
189             if not t1.must_hold:
190                 t1.must_hold=True
191                 checklist.append(t1)
192     t.consequences=[]
193 for t in restrictions:
194     for t1 in t.consequences:
195         if not t1 in restrictions:restrictions.append(t1)

```

Each abstract occupied level is attributed a list of all conditions of the form  $\langle xyz \rangle$  involving it.

```

196 for t in restrictions:
197     for x in t:
198         x.conditions.append(t)

```

Now we prepare the initial state of the instruments operated during the search.

Abstract occupied occupied levels that are not assigned a definite position are organized into a priority queue. The smaller number of elements in the `options` attribute of an abstract occupied level the higher priority it has. The queue is implemented as a dictionary that associates with every  $k \in \mathbb{N}$  a list of all occupied levels with the length of the `options` list equal to  $k$  provided that the list is not empty.

The initial order in which we put the abstract occupied levels into the queue does not affect the result, but it can affect the efficiency. The principle that has been chosen is this: for any  $i \geq 2$  there must exist  $j < i$  such that some rectangle has its sides on both occupied levels that take the  $i$ th and the  $j$ th positions in the queue. In the sequel, we use the LIFO rule for entries of equal priority.

```

199 pos=hposition.registry[0]
200 q=[pos]
201 for p in q:
202     for r in p.rectangles:
203         for side in ['left','right','top','bottom']:
204             p1=r.__dict__[side]
205             if not p1 in q:q.append(p1)
206 queuedict={1:q}

```

The `li` attribute of the `hposition` and `vposition` classes holds the respective list of abstract occupied levels that are currently assigned a definite position. The remaining abstract occupied levels are put in `unsetposlist`.

```

207 hposition.li=[]
208 vposition.li=[]
209 unsetposlist=list(q)

```

The `actionstack` list is a stack where we record all our actions that are eventually to be undone. The realizations that are found during the search are put into the `realizations` list.

```

210 actionstack=[]
211 realizations=[]

```

A couple of counters for user's information...

```

212 numoftries=0
213 numofdestabilizable=0

```

... and a few constants for better readability.

```

214 (assume,delopt,addopt,switch)=range(0,4)

```

Here are the functions to operate the queue.

```

215 def get_from_queue():
216     global queuedict
217     qkeys=queuedict.keys()
218     minq=min(qkeys)
219     p=queuedict[minq].pop(0)
220     if len(queuedict[minq])==0:del queuedict[minq]
221     return p
222 def put_to_queue(p):
223     global queuedict
224     k=len(p.options)
225     if not k in queuedict:queuedict[k]=[]
226     queuedict[k].insert(0,p)
227 def delete_option(p,i):
228     if len(p.options)==1:raise Contradiction
229     global queuedict
230     k=len(p.options)
231     queuedict[k].remove(p)
232     if len(queuedict[k])==0:del queuedict[k]
233     del p.options[i]
234     if not k-1 in queuedict:queuedict[k-1]=[]
235     queuedict[k-1].insert(0,p)
236 def restore_option(p,i,place):
237     global queuedict
238     k=len(p.options)
239     queuedict[k].remove(p)
240     if len(queuedict[k])==0:del queuedict[k]
241     p.options.insert(i,place)
242     if not k+1 in queuedict:queuedict[k+1]=[]
243     queuedict[k+1].insert(0,p)

```

Here starts the main loop.

```

244 while True:
245     try:

```

Get an abstract occupied level from the queue and put it to the first available position. Put a record to the action stack that we made an assumption on the position of this occupied level.

```

246     currpos=get_from_queue()
247     currposclass=currpos.__class__
248     place=currpos.options[0]
249     actionstack.append((assume,currpos))
250     currposclass.li.insert(place,currpos)
251     currpos.place=place
252     unsetposlist.remove(currpos)

```

The `place` attribute of each abstract occupied level on the position of which an assumption has been made coincides with its index in the `li` list attributed to the corresponding `position` subclass. When we insert an element into this list, the subsequent indices are shifted, so, we take care of the `place` attribute of the corresponding entries.

```

253     for p in currposclass.li[place+1:]:
254         p.place+=1

```

The entries in the `option` lists of abstract occupied levels that are not yet assigned a concrete position must be adjusted accordingly.

```

255     for p in unsetposlist:
256         if p.__class__==currposclass:
257             o=p.options
258             i=0
259             while i<len(o):
260                 j=o[i]
261                 if j==place and j>0:
262                     actionstack.append((adopt,p,i))
263                     restore_option(p,i,place)
264                     i+=1
265                 if j>=place:
266                     o[i]+=1
267                 i+=1

```

All first order conditions that involve the occupied level on the position of which we have just made an assumption are now to be upgraded.

```

268     for rest in currpos.conditions:
269         rest.level+=1

```

If there are no entries in the `unsetposlist` list left it means we have found a realization. We append it to the `realizations` list unless the boundary of the diagram is destabilizable.

```

270     if len(unsetposlist)==0:
271         hp=hposition.li
272         vp=vposition.li
273         hedgeposlist=[hp.index(h) for (h,v1,v2) in ve]
274         hedgeposlist.sort()
275         vedgeposlist=[vp.index(v) for (v,h1,h2) in he]
276         vedgeposlist.sort()
277         hp1=[(vp.index(v),hp.index(h1),hp.index(h2)) for\
278             (v,h1,h2) in he]
279         hp1.sort()
280         vp1=[(hp.index(h),vp.index(v1),vp.index(v2)) for\

```

```

281         (h,v1,v2) in ve]
282     vp1.sort()
283     n=len(hp1)
284     for (v,h1,h2) in hp1:
285         if (hedgeposlist.index(h1)-hedgeposlist.index(h2))%n\
286             in (1,n-1):
287             numofdestabilizable+=1
288             raise Contradiction
289     for (h,v1,v2) in vp1:
290         if (vedgeposlist.index(v1)-vedgeposlist.index(v2))%n\
291             in (1,n-1):
292             numofdestabilizable+=1
293             raise Contradiction
294     realizations.append((list(hposition.li),
295                          list(vposition.li)))
296     raise Contradiction

```

Now we derive consequences from our last assumption. We collect all first order conditions whose `level` has just reached 2 into the `apply_restrictions` list. Also, for any second order condition  $\langle abc \rangle \Rightarrow \langle xyz \rangle$  such that the level of  $\langle abc \rangle$  has just turned 3 we evaluate  $\langle abc \rangle$ , and if the result is `True`, we turn  $\langle xyz \rangle$  into a first order condition, and make a record about this into the action stack. If the level of this condition has just reached 2 we add it to the `apply_restrictions` list.

```

297     apply_restrictions=[]
298     for rest in currpos.conditions:
299         if rest.level==2 and rest.must_hold:
300             apply_restrictions.append(rest)
301         elif rest.level==3 and len(rest.consequences)>0:
302             (k,l,m)=(p.place for p in rest)
303             if even(k,l,m):
304                 for con in rest.consequences:
305                     if not con.must_hold:
306                         actionstack.append((switch,con))
307                         con.must_hold=True
308                     if con.level==2:
309                         apply_restrictions.append(con)

```

Now the `apply_restrictions` list consists of first order conditions  $\langle abc \rangle$  such that exactly two of the three abstract occupied levels  $a, b, c$  are assigned a concrete position, and the third one is not. We adjust the available places for this, third, abstract occupied level by discarding those that violate the condition  $\langle abc \rangle$ . As always, a record about this is made on the action stack.

```

310     for rest in apply_restrictions:
311         x=tuple(p.place for p in rest)
312         j=x.index(None)
313         k=x[(j+1)%3]
314         l=x[(j-1)%3]
315         p=rest[j]
316         o=p.options
317         i=0
318         while i<len(o):

```

```

319         m=o[i]
320         if not m==1 and (m==k or even(k,l,m)):
321             i+=1
322         else:
323             delete_option(p,i)
324             actionstack.append((delopt,p,i,m))

```

When a `Contradiction` exception is raised we undo the last actions recorded in the action stack until the last essential assumption is encountered. The list of available places for the abstract occupied level on which that assumption is made is modified by deleting the corresponding option so the same assumption is not immediately made again. This deletion is reflected in the action stack so, when all options have been tried and the previous essential assumption is to be withdrawn, the available places for this abstract occupied level are recovered.

```

325     except Contradiction:
326         numoftries+=1
327         while len(actionstack)>0:
328             action=actionstack.pop(-1)
329             if action[0]==assume:
330                 currpos=action[1]
331                 place=currpos.place
332                 currposclass=currpos.__class__
333                 for rest in currpos.conditions:
334                     rest.level-=1
335                 for p in unsetposlist:
336                     if p.__class__==currposclass:
337                         o=p.options
338                         i=0
339                         while i<len(o):
340                             j=o[i]
341                             if j>place:o[i]-=1
342                             i+=1
343                 for p in currposclass.li[place+1:]:
344                     p.place-=1
345                 unsetposlist.insert(0,currpos)
346                 currpos.place=None
347                 del currposclass.li[place]
348                 put_to_queue(currpos)
349                 if len(currpos.options)>1:
350                     actionstack.append((delopt,currpos,0,place))
351                     delete_option(currpos,0)
352                     break
353                 elif action[0]==delopt:
354                     (p,i,place)=action[1:]
355                     restore_option(p,i,place)
356                 elif action[0]==addopt:
357                     (p,i)=action[1:]
358                     delete_option(p,i)
359                 elif action[0]==switch:
360                     con=action[1]
361                     con.must_hold=False

```

When the action stack is empty the search finishes.

```
362     if len(actionstack)==0:break
```

Some information about the work having been done is displayed.

```
363 print('number of cases considered',numoftries)
364 print('number of realizations found',len(realizations))
365 print('number of destabilizable diagrams found',numofdestabilizable)
```

Now the output file is going to be written. The format of the file is discussed in the next section.

```
366 prefix=open('prefix.txt','r')
367 pre=prefix.readlines()
368 prefix.close()
369 output=open('realizations.eps','w')
370 for s in pre:output.write(s)
371 nh=len(hposition.registry)
372 nv=len(vposition.registry)
373 for (hp,vp) in realizations:
374     output.write('/shift [0 0] def\n')
375     output.write('/gridsize [%s %s] def\n/rectangles\n['%(nh,nv))
376     j=0
377     for i in rectangle.registry:
378         j+=1
379         r=rectangle.registry[i]
380         output.write('%s %s %s %s (%s) '\
381                     %(hp.index(r.left),hp.index(r.right),\
382                       vp.index(r.bottom),vp.index(r.top),r.label))
383         if j%5==0:output.write('\n')
384     output.write('] def\n')
385     output.write('/hedges\n[')
386     for (v,h1,h2) in he:
387         output.write('%s %s %s'%(vp.index(v),hp.index(h1),\
388                                 hp.index(h2)))
389     output.write('] def\n')
390     output.write('/vedges\n[')
391     for (h,v1,v2) in ve:
392         output.write('%s %s %s'%(hp.index(h),vp.index(v1),\
393                                 vp.index(v2)))
394     output.write('] def\n')
395     output.write('drawall\nshowpage\n')
396 output.write('%%EOF\n')
397 output.close()
```

#### 4. OUTPUT

The output of the script is written into the `realizations.eps` file. It is supposed to be a multi-page Encapsulated PostScript file, which is officially not legitimate, though certain software does not mind to display it in the multi-page mode. Other software will show only the first page. The user can edit the output file by any simple text editor to meet his or her requirements.



The output file starts from a preamble, which is just copied from the file `prefix.txt`. This file is a part of the package, it contains the definition of a script called `drawall` doing all the graphic job. The contents of the file are shown in the Appendix without further comments.

Then the page descriptions follow, each page representing a single diagram. Pages are separated by the `showpage` command. The description of each page consists of five array definitions followed by the `drawall` command, for instance:

```
/shift [0 0] def
/gridsize [14 14] def
/rectangles
[13 0 9 0 (1) 0 3 0 4 (2) 3 10 4 6 (3) 10 11 6 13 (4) 4 5 1 7 (5)
5 6 7 11 (6) 2 5 11 12 (7) 5 9 12 13 (8) 9 10 13 3 (9) 10 12 3 4 (10)
12 0 4 7 (11) 0 4 7 9 (12) 6 8 2 7 (13) 8 12 7 8 (14) 3 5 13 0 (15)
5 7 0 1 (16) 7 8 8 0 (17) 8 13 0 2 (18) 9 1 10 12 (19) 1 2 12 5 (20)
11 1 5 6 (21) 1 3 6 10 (22) ] def
/hedges
[9 13 4 13 3 11 1 4 7 11 2 6 3 9 12 2 6 13 8 7 12 10 9 3 5 11 2 ] def
/vedges
[13 9 2 3 13 10 11 5 13 4 1 9 6 2 11 2 11 5 9 10 3 12 3 8 7 8 1 ] def
drawall
```

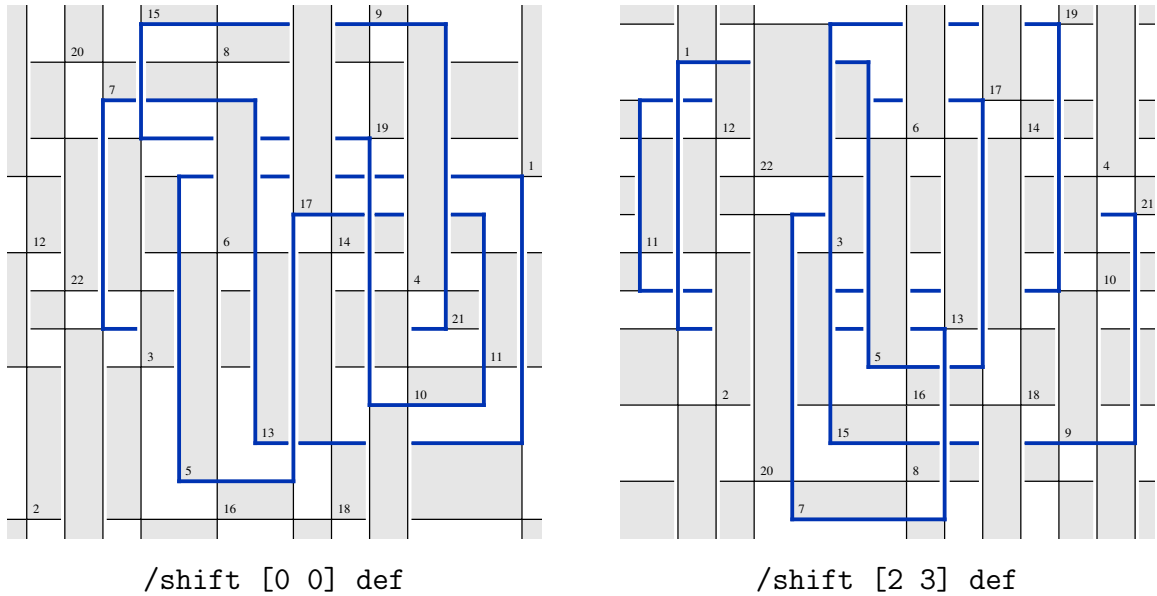

FIGURE 3. Sample output

The corresponding diagram is shown in Figure 3 on the left. The precise meaning of these arrays is as follows.

The `gridsize` array keeps the numbers of horizontal and vertical occupied levels (these numbers are not necessarily equal).

The `shift` array is always set to `[0 0]` and is supposed to be changed manually by the user if necessary. Put any non-negative integers here and the whole diagram will be shifted accordingly. The shift is regarded modulo `gridsize`, but the picture will be transformed properly only if both entries of the `shift` array are non-negative. The right picture in Figure 3 shows the result of the shift by the vector  $(2, 3)$ .

The `rectangles` array contains the rectangle data. A rectangle  $[a; b] \times [c; d]$  labelled ‘ $e$ ’ is encoded as `a b c d (e)`.

The `hedges` and `vedges` lists keep the lists of horizontal and vertical edges, respectively, of the boundary of the diagram. A horizontal (respectively, vertical) edge with endpoints  $(b, a)$  and  $(c, a)$  (respectively,  $(a, b)$  and  $(a, c)$ ) is encoded as `a b c`.

## 5. CONCLUDING REMARKS

**5.1.** The labels of the rectangles need not be consecutive natural numbers, one may use any numbers or strings.

**5.2.** The script does not check the initial data for consistency. It is required that the dividing code correspond to a dividing configuration  $(\delta_+, \delta_-)$  on a surface  $F$  such that each connected component of  $\partial F$  meets  $\delta_+ \cup \delta_-$  in at least four points. This condition is necessary for a realization to exist, and if it is not satisfied, the output of the script may not be sensible or a runtime error may occur.

**5.3.** The algorithm implemented by the present script is not completely deterministic, and the outputs of different runs of the script may differ in the order in which the diagrams follow. The number of considered cases, which is displayed on the screen at the end of the process, may also vary. This is because, in lines 107, 127, 137, and 139, we let a variable run over a set in the order chosen at Python interpreter’s discretion.

This can easily be changed, but the motivation for that has not been strong enough. Moreover, this randomness of the process is a useful feature for ensuring that there are no bugs in the program (and for revealing them if they were present) by comparing the results of several different runs of the program for the same initial data.

**5.4.** Another method of searching all realizations of a dividing code had been tried by the author prior to writing this script. The method was to search all orderings of horizontal occupied levels that satisfy all first order conditions, then do the same for vertical occupied levels, and finally check which pairs of orderings satisfy all second order conditions.

This method appears to be much less efficient than the one described in the present note. The point is that the number of orderings of occupied levels of a chosen direction, vertical or horizontal, satisfying all first order conditions is typically much larger than the number of search rounds made by the present script.

## APPENDIX: THE FILE `prefix.txt`

```

1 %!PS-Adobe-3.1 EPSF-3.0
2 %%BoundingBox: 0 0 420 420
3 /datasize 5 def
4
5 /drawall
6 {10 10 translate
7  newpath 0 0 moveto 400 0 rlineto 0 400 rlineto
8  -400 0 rlineto closepath clip
9  /maxgridsize gridsize 0 get gridsize 1 get
10 gt
11 {gridsize 0 get
12 }
13 {gridsize 1 get
14 } ifelse def
15 400 30 maxgridsize mul div dup scale
16 /hstep maxgridsize gridsize 0 get div 30 mul def

```

```

17 /vstep maxgridsize gridsize 1 get div 30 mul def
18 /lmargin hstep neg def
19 /rmargin gridsize 0 get hstep mul def
20 /bmargin vstep neg def
21 /tmargin gridsize 1 get vstep mul def
22 /rectangles
23 [0 datasize rectangles length 1 sub
24   {/k exch def
25     /i1 rectangles k get shift 0 get add gridsize 0 get mod def
26     /i2 rectangles k 1 add get shift 0 get add gridsize 0 get mod def
27     /j1 rectangles k 2 add get shift 1 get add gridsize 1 get mod def
28     /j2 rectangles k 3 add get shift 1 get add gridsize 1 get mod def
29     i1 i2 lt
30     {i1 i2 j1 j2 k 4 add 1 k datasize add 1 sub
31       {rectangles exch get
32       } for
33     }
34     {i1 i2 gridsize 0 get add j1 j2 k 4 add 1 k datasize add 1 sub
35       {rectangles exch get
36       } for
37     i1 gridsize 0 get sub i2 j1 j2 k 4 add 1 k datasize add 1 sub
38     {rectangles exch get
39     } for
40   } ifelse
41 } for
42 ] def
43 /rectangles
44 [0 datasize rectangles length 1 sub
45   {/k exch def
46     /i1 rectangles k get def
47     /i2 rectangles k 1 add get def
48     /j1 rectangles k 2 add get def
49     /j2 rectangles k 3 add get def
50     j1 j2 lt
51     {i1 i2 j1 j2 k 4 add 1 k datasize add 1 sub
52       {rectangles exch get
53       } for
54     }
55     {i1 i2 j1 gridsize 1 get sub j2 k 4 add 1 k datasize add 1 sub
56       {rectangles exch get
57       } for
58     i1 i2 j1 j2 gridsize 1 get add k 4 add 1 k datasize add 1 sub
59     {rectangles exch get
60     } for
61   } ifelse
62 } for
63 ] def
64 /hedges
65 [0 3 hedges length 1 sub
66   {/k exch def
67     hedges k get shift 1 get add gridsize 1 get mod
68     /i1 hedges k 1 add get shift 0 get add gridsize 0 get mod def
69     /i2 hedges k 2 add get shift 0 get add gridsize 0 get mod def
70     i1 i2 lt {i1 i2} {i2 i1} ifelse
71   } for
72 ] def
73 /vedges

```

```

74 [0 3 vedges length 1 sub
75   {/k exch def
76     vedges k get shift 0 get add gridsize 0 get mod
77     /i1 vedges k 1 add get shift 1 get add gridsize 1 get mod def
78     /i2 vedges k 2 add get shift 1 get add gridsize 1 get mod def
79     i1 i2 lt {i1 i2} {i2 i1} ifelse
80   } for
81 ] def
82 0.5 hstep mul 0.5 vstep mul translate
83 0 datasize rectangles length 1 sub
84 {/k exch def
85   /i1 rectangles k get def
86   /i2 rectangles k 1 add get def
87   /j1 rectangles k 2 add get def
88   /j2 rectangles k 3 add get def
89   gsave
90   0 datasize rectangles length 1 sub
91   {/l exch def
92     /ii1 rectangles l get def
93     /ii2 rectangles l 1 add get def
94     /jj1 rectangles l 2 add get def
95     /jj2 rectangles l 3 add get def
96     i1 ii1 lt ii2 i2 lt jj1 j1 lt j2 jj2 lt and and and
97     {newpath lmargin bmargin moveto
98       ii1 hstep mul 3 sub bmargin lineto
99       ii1 hstep mul 3 sub tmargin lineto
100      lmargin tmargin lineto closepath
101      rmargin bmargin moveto
102      ii2 hstep mul 3 add bmargin lineto
103      ii2 hstep mul 3 add tmargin lineto
104      rmargin tmargin lineto closepath clip
105     } if
106   } for
107   0 3 vedges length 1 sub
108   {/l exch def
109     /ii vedges l get def
110     /jj1 vedges l 1 add get def
111     /jj2 vedges l 2 add get def
112     i1 ii lt ii i2 lt jj1 j1 lt j2 jj2 lt and and and
113     {newpath lmargin bmargin moveto
114       ii hstep mul 4 sub bmargin lineto
115       ii hstep mul 4 sub tmargin lineto
116       lmargin tmargin lineto closepath
117       rmargin bmargin moveto
118       ii hstep mul 4 add bmargin lineto
119       ii hstep mul 4 add tmargin lineto
120       rmargin tmargin lineto closepath clip
121     } if
122   } for
123   newpath
124   i1 hstep mul j1 vstep mul moveto
125   i2 hstep mul j1 vstep mul lineto
126   i2 hstep mul j2 vstep mul lineto
127   i1 hstep mul j2 vstep mul lineto
128   closepath gsave 0.9 setgray fill grestore stroke
129   i1 hstep mul 5 add j1 vstep mul 5 add moveto
130   /Times-Roman findfont 10 scalefont setfont rectangles

```

```

131     k 4 add get show
132     grestore
133 } for
134 newpath
135 0 3 vedges length 1 sub
136 {/k exch def
137     vedges k get hstep mul
138     vedges k 1 add get vstep mul moveto
139     0 vedges k 2 add get vedges k 1 add get sub vstep mul rlineto
140 } for
141 3 setlinewidth 2 setlinecap 0 0.2 0.7 setrgbcolor stroke
142 0 3 hedges length 1 sub
143 {/k exch def
144     /j hedges k get def
145     /i1 hedges k 1 add get def
146     /i2 hedges k 2 add get def
147     gsave
148     0 datasize rectangles length 1 sub
149     {/l exch def
150         /ii1 rectangles l get def
151         /ii2 rectangles l 1 add get def
152         /jj1 rectangles l 2 add get def
153         /jj2 rectangles l 3 add get def
154         i1 ii1 lt ii2 i2 lt jj1 j lt j jj2 lt and and and
155         {newpath lmargin bmargin moveto
156             ii1 hstep mul 3 sub bmargin lineto
157             ii1 hstep mul 3 sub tmargin lineto
158             lmargin tmargin lineto closepath
159             rmargin bmargin moveto
160             ii2 hstep mul 3 add bmargin lineto
161             ii2 hstep mul 3 add tmargin lineto
162             rmargin tmargin rlineto closepath clip
163         } if
164     } for
165     0 3 vedges length 1 sub
166     {/l exch def
167         /ii vedges l get def
168         /jj1 vedges l 1 add get def
169         /jj2 vedges l 2 add get def
170         i1 ii lt ii i2 lt jj1 j lt j jj2 lt and and and
171         {newpath lmargin bmargin moveto
172             ii hstep mul 4 sub bmargin lineto
173             ii hstep mul 4 sub tmargin lineto
174             lmargin tmargin lineto closepath
175             rmargin bmargin moveto
176             ii hstep mul 4 add bmargin lineto
177             ii hstep mul 4 add tmargin lineto
178             rmargin tmargin rlineto closepath clip
179         } if
180     } for
181     newpath
182     i1 hstep mul j vstep mul moveto
183     i2 i1 sub hstep mul 0 rlineto
184     stroke
185     grestore
186 } for
187 } def

```

---

## REFERENCES

- [1] I. Dynnikov, M. Prasolov. Rectangular diagrams of surfaces: representability, *Matem. Sb.* **208** (2017), no. 6, 55–108; translation in *Sb. Math.* **208** (2017), no. 6, 781–841, arXiv:1606.03497.
- [2] I. Dynnikov, M. Prasolov. Rectangular diagrams of surfaces: distinguishing Legendrian knots. *Preprint*, arXiv:1712.06366.

V.A. STEKLOV MATHEMATICAL INSTITUTE OF RUSSIAN ACADEMY OF SCIENCE, 8 GUBKINA STR., MOSCOW 119991, RUSSIA

*E-mail address:* dynnikov@mech.math.msu.su
